# Supplementary material for: Quality Matters: Evaluating Synthetic Data for Tool-Using LLMs
Source: arXiv:2409.16341 source file (2024-09-26)
Supplement: Supplementary file 1 [file appendix_prompts.tex]

% \begin{table}[htbp]
%     \centering
%     \begin{tabular}{|c|c|c|c|c|c|}
%     \hline
%     Metric & Accuracy & Precision & Recall & F1  \\
%     \hline
%     specificity & 0.54 & 0.56 & 0.36 & 0.43  \\
%     \hline
%     \end{tabular}
%     \caption{Metrics}
%     \label{tab:}
% \end{table}


% \begin{table}[htbp]
%     \centering
%     \begin{tabular}{|c|c|c|c|c|c|}
%     \hline
%     Metric & Accuracy & Precision & Recall & F1  \\
%     \hline
%     coherence & 0.74 & 0.5	& 0.46 & 0.48  \\
%     \hline
%     \end{tabular}
%     \caption{Metrics}
%     \label{tab:}
% \end{table}



% \subsubsection{Coherence - Ranking}

% \begin{figure}[h]
%   \centering
%   \includegraphics[width=\linewidth]{figures/prompt_coherence_direct.png}
%   \caption{Prompt for Coherence - Direct Questioning. % COMMENT \shadi{What do you think of this?}
%   }
%   \label{fig:prompt_coherence_direct}
% \end{figure}

% \subsubsection{Coherence - NSP}


% \begin{figure}[h]
%   \centering
%   \includegraphics[width=\linewidth]{figures/prompt_coherence_task.png}
%   \caption{Prompt for Coherence - Next Sentence Coherence Prediction Task. 
%   }
%   \label{fig:prompt_coherence_task}
% \end{figure}

% \subsubsection{Solvable}

% \begin{figure}[h]
%   \centering
%   \includegraphics[width=\linewidth]{figures/prompt_solvable_direct.png}
%   \caption{Prompt for Solvable - Direct Questioning. % COMMENT \shadi{What do you think of this?}
%   }
%   \label{fig:prompt_solvable_direct}
% \end{figure}

% \subsubsection{Parameters Alignment  - Direct}

% \begin{figure}[h]
%   \centering
%   \includegraphics[width=\linewidth]{figures/prompt_param_direct.png}
%   \caption{Prompt for Parameters Alignment - Direct Questioning. 
%   }
%   \label{fig:prompt_param_direct}
% \end{figure}


% \subsubsection{Parameters Matching - Extraction Task}

% \begin{figure}[h]
%   \centering
%   \begin{subfigure}{\linewidth}
%     \centering
%     \includegraphics[width=0.8\linewidth]{figures/prompt_param_extract1.png}
%     \caption{Step 1: Extraction Task.}
%     \label{fig:prompt_param_extract1}
%   \end{subfigure}
  
%   \begin{subfigure}{\linewidth}
%     \centering
%     \includegraphics[width=0.8\linewidth]{figures/prompt_param_compare2.png}
%     \caption{Step 2: Comparison.}
%     \label{fig:prompt_param_compare2}
%   \end{subfigure}
  
%   \caption{Prompt for Parameters Alignment - NLP tasking.}
%   \label{fig:prompt_param_task}
% \end{figure}

% \subsubsection{Matching API sequence + Minimal API calls}

% \begin{figure}[h]
%   \centering
%   \includegraphics[width=\linewidth]{figures/prompt_api.png}
%   \caption{Prompt for API Matching and Minimal Calls. 
%   }
%   \label{fig:prompt_api}
% \end{figure}
