# Supplementary material for: Quality Matters: Evaluating Synthetic Data for Tool-Using LLMs
Source: arXiv:2409.16341 source file (2024-09-26)
Supplement: Supplementary file 2 [file appendix_prompts_old.tex]

% \shadi{I'm just putting the prompt/results here. Will show it as figures later on.}

% \subsubsection{Specificity - Rating Prompt}
% \texttt{You are a helpful data quality researcher. You will be given data examples which are generated by an AI model for the goal of training an AI assistant to use API tools. Each data example is an instruction which should resemble real-world scenarios.
% Your task is to estimate each instruction quality in terms of completeness and specificity.
% Evaluate the specificity of each instruction, considering whether it contains all necessary information without gaps for the AI assistant to respond with a use of an external function call. The parameter values should be mentioned explicitly.
% Use a scale from 1 to 5 for assessment, with 1 being the lowest score and 5 the highest.
% 1 (Poor): The instruction is broad and general, lacks essential details.
% 2 (Limited): The instruction is general, lacks specific information.
% 3 (Average): The instruction includes moderate specific details, but there are some gaps in information.
% 4 (Good): The instruction is reasonably complete, with only minor missing details.
% 5 (Excellent): The instructions are highly specific and complete, with no significant missing information.
% Example 1:
% Query: "Can you fetch the flight data for the company AZU on June 15th, 2022?"
% Required Parameters: [company, date]
% Start Answer:
% Query explanation: the company name and date are mentioned explicitly. 
% Score: 5 (Excellent)
% Example 2:
% Query: "Can you fetch the flight data for the company ?"
% Required Parameters: [company, date]
% Query explanation: the company name and date are not mentioned explicitly. 
% Score: 1 (Poor)
% }


% \begin{table}[htbp]
%     \centering
%     \begin{tabular}{|c|c|c|c|c|c|}
%     \hline
%     Metric & Accuracy & Precision & Recall & F1  \\
%     \hline
%     specificity & 0.50 & 0.50 & 0.44 & 0.47  \\
%     \hline
%     \end{tabular}
%     \caption{Metrics}
%     \label{tab:}
% \end{table}


\subsubsection{Specificity - Direct Questioning}

% \texttt{
% You are a helpful data quality researcher. You will be given data examples which are generated by an AI model for the goal of training an AI assistant to use API tools. Each data example is an instruction which should resemble real-world scenarios.
% Your task is to estimate each instruction quality in terms of completeness and specificity.
% Evaluate the specificity of each instruction, considering whether it contains all necessary information without gaps for the AI assistant to respond with a use of an external function call.
% Answer with (Specific/Unspecific)
% Specific: The instruction is highly specific and complete, with no significant missing information. The parameters values are mentioned explicitly.
% Unspicific: The instruction lacks essential details or variables. The parameters values are not mentioned explicitly.
% Example 1:
% Query: "Can you fetch the flight data for the company AZU on June 15th, 2022?"
% Required Parameters: [company, date]
% Start Answer:
% Query explanation: the company name and date are mentioned explicitly.
% Answer: Specific
% Example 2:
% Query: "Can you fetch the flight data for the company ?"
% Required Parameters: [company, date]
% Query explanation: the company name and date are not mentioned explicitly.
% Answer: Unspecific
% }

\begin{figure}[h]
  \centering
  \includegraphics[width=\linewidth]{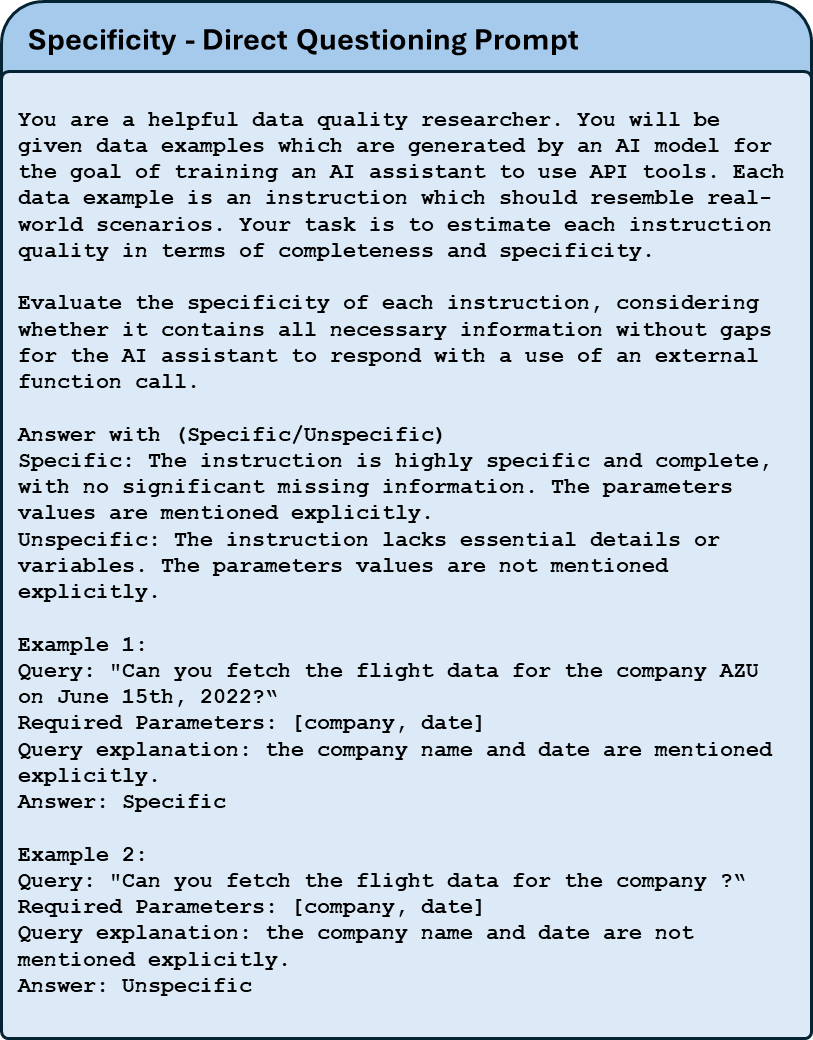}
  \caption{Prompt for Specificity - Direct Questioning. % COMMENT \shadi{What do you think of this?}
  }
  \label{fig:prompt_specificity_direct}
\end{figure}

\begin{table}[htbp]
    \centering
    \begin{tabular}{|c|c|c|c|c|c|}
    \hline
    Metric & Accuracy & Precision & Recall & F1  \\
    \hline
    specificity & 0.54 & 0.56 & 0.36 & 0.43  \\
    \hline
    \end{tabular}
    \caption{Metrics}
    \label{tab:}
\end{table}


\subsubsection{Specificity - Extraction Task}

% \texttt{
% You are data quality researcher in natural language. You have two tasks to do one after the other.
% I will give you user instruction to an AI assistant. This instruction might include one or more requests. 
% Focus on the requests the user make, then 1) Think of required parameters the AI assistant might need in order to fulfill the user request. It could be None.
% and 2) Extract the parameter values from the instruction. Choose only important parameters required for the API, if there are any. 
% Use \#missing for parameter values that are not explicitly provided in the query. 
% Example 1:
% Query: "Can you fetch the flight data for the company AZU on June 15th, 2022?"
% Required Parameters: [company, date]
% Start Answer:
% company = 'AZU'
% date = 'June 15th, 2022' 
% Example 2:
% Query: "Can you fetch the flight data for the company ?"
% Required Parameters: [company, date]
% Start Answer:
% company = \#missing
% date = \#missing
% Queries: }

\begin{figure}[h]
  \centering
  \includegraphics[width=\linewidth]{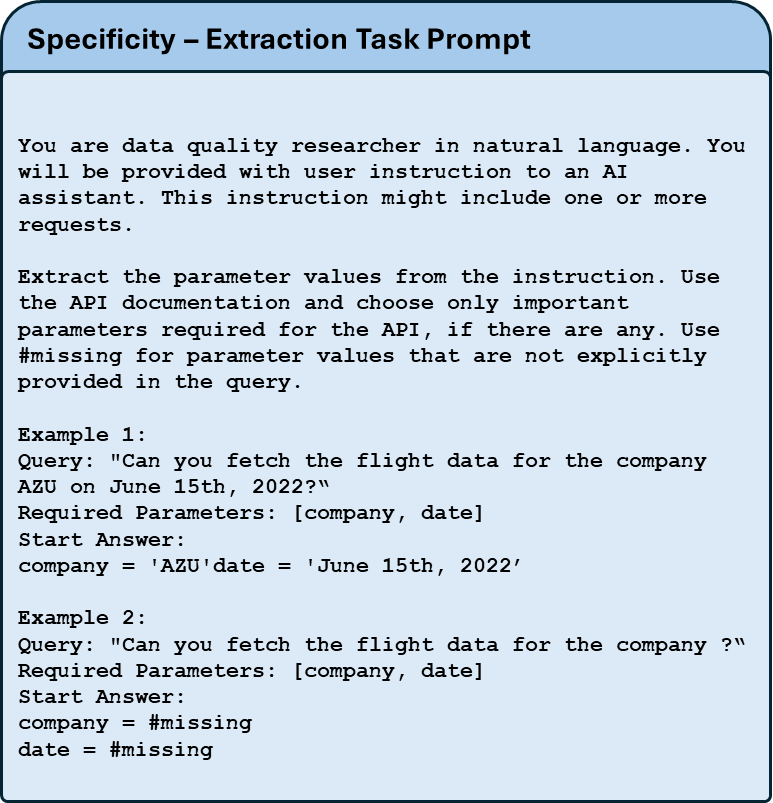}
  \caption{Prompt for Specificity - Extraction Task.
  }
  \label{fig:prompt_specificity_task}
\end{figure}



\subsubsection{Coherence - Ranking}
% \texttt{
% You are a helpful data quality researcher. You will be given data examples which are generated by an AI model for the goal of training an AI assistant to use API tools. Each data example is a single or multi instructions which should resemble real-world scenarios.
% Your task is to estimate each instruction quality in terms of coherence.
% Evaluate the extent to which the different requests or components of the instruction are logically connected and relevant to each others.
% Use a scale from 1 to 5 for assessment, with 1 being the lowest score and 5 the highest.
% 1 (Poor): The components or different requests of the instruction are highly disjointed, lacking a logical connection.
% 2 (Limited): The components or different requests of the instruction are somewhat related but exhibit notable separation.
% 3 (Average): The components or different requests of the instruction have a moderate level of coherence but still possess some degree of separation.
% 4 (Good): The components or different requests of the instruction are reasonably connected and logically related.
% 5 (Excellent): The components or different requests of the instruction are highly coherent, with a strong logical connection.
% Examples:
% Query: I'm a cryptocurrency trader, and I want to analyze the historical prices and market caps of popular cryptocurrencies like Bitcoin, Ethereum, and Stellar. Can you fetch this information for me using the Crypto Prices API? Additionally, I'm planning a trip to North America and I would like to know the subregions in North America using the Geography API.
% Explanation: Fetching crypto information is not related to fetching geography information request.
% Score = 1 (Poor).
% Query: I want to impress my friends with some hilarious jokes. Can you fetch some Chuck Norris jokes related to 'sports'? Also, fetch me some Chuck Norris jokes related to 'art'?
% Explanation: The different requests in the instruction are all related to jokes.
% Score = 5 (Excellent)
% }
\begin{figure}[h]
  \centering
  \includegraphics[width=\linewidth]{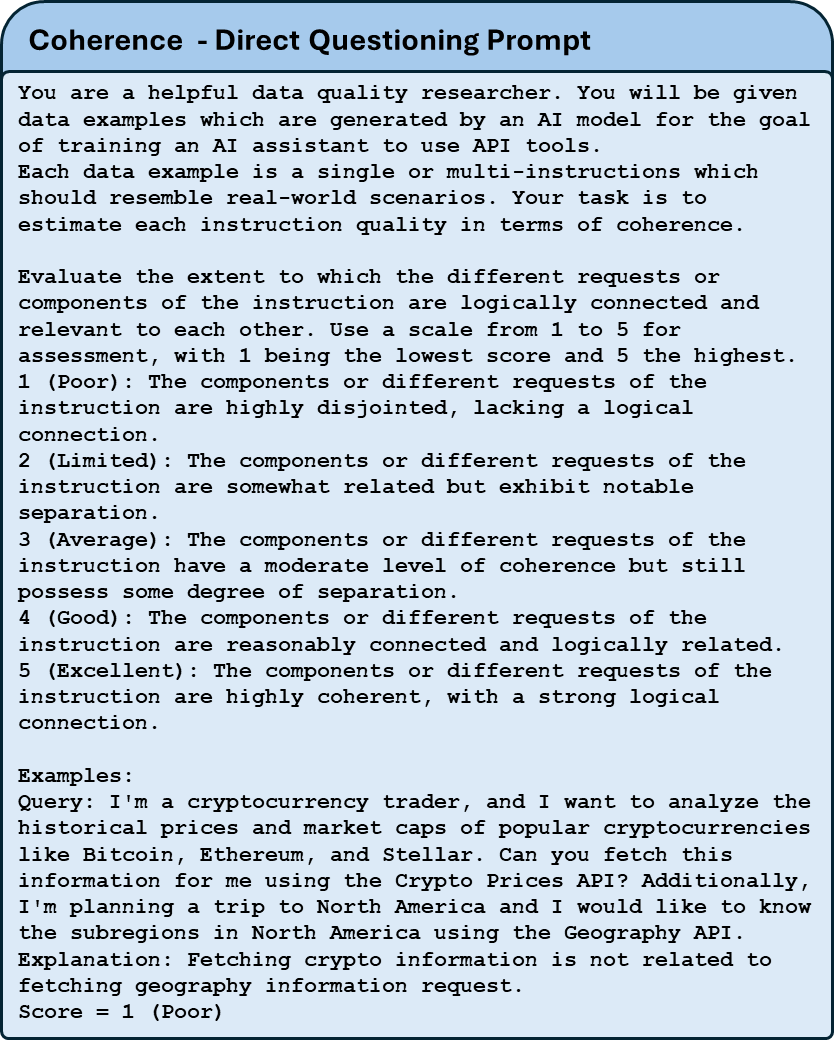}
  \caption{Prompt for Coherence - Direct Questioning. % COMMENT \shadi{What do you think of this?}
  }
  \label{fig:prompt_coherence_direct}
\end{figure}

\begin{table}[htbp]
    \centering
    \begin{tabular}{|c|c|c|c|c|c|}
    \hline
    Metric & Accuracy & Precision & Recall & F1  \\
    \hline
    coherence & 0.74 & 0.5	& 0.46 & 0.48  \\
    \hline
    \end{tabular}
    \caption{Metrics}
    \label{tab:}
\end{table}


\subsubsection{Coherence - NSP}

% \texttt{
% You are tasked with assess the contextual coherence between pairs of sentences.
% Contextual coherence refers to the likelihood that the second sentence follows the first sentence in a coherent and logical manner.
% For each pair of consecutive sentences, predict whether the second sentence is likely to follow the first sentence in a coherent sequence. Consider the flow of information and whether the second sentence is contextually appropriate following the first sentence.
% Examples:
% Query: 
% 1. "I'm a cryptocurrency trader, and I want to analyze the historical prices and market caps of popular cryptocurrencies like Bitcoin, Ethereum, and Stellar."
% 2. "Can you fetch this information for me using the Crypto Prices API?"
% 3. "Additionally, I'm planning a trip to North America and I would like to know the subregions in North America using the Geography API."
% Answer:
% 1-2 = coherent
% 2-3 = incoherent
% Query: 
% 1. I want to impress my friends with some hilarious jokes.
% 2. Can you fetch some Chuck Norris jokes related to 'sports'?
% 3. Also, fetch me some Chuck Norris jokes related to 'art'?
% Answer:
% 1-2 = coherent
% 2-3 = coherent
% }

\begin{figure}[h]
  \centering
  \includegraphics[width=\linewidth]{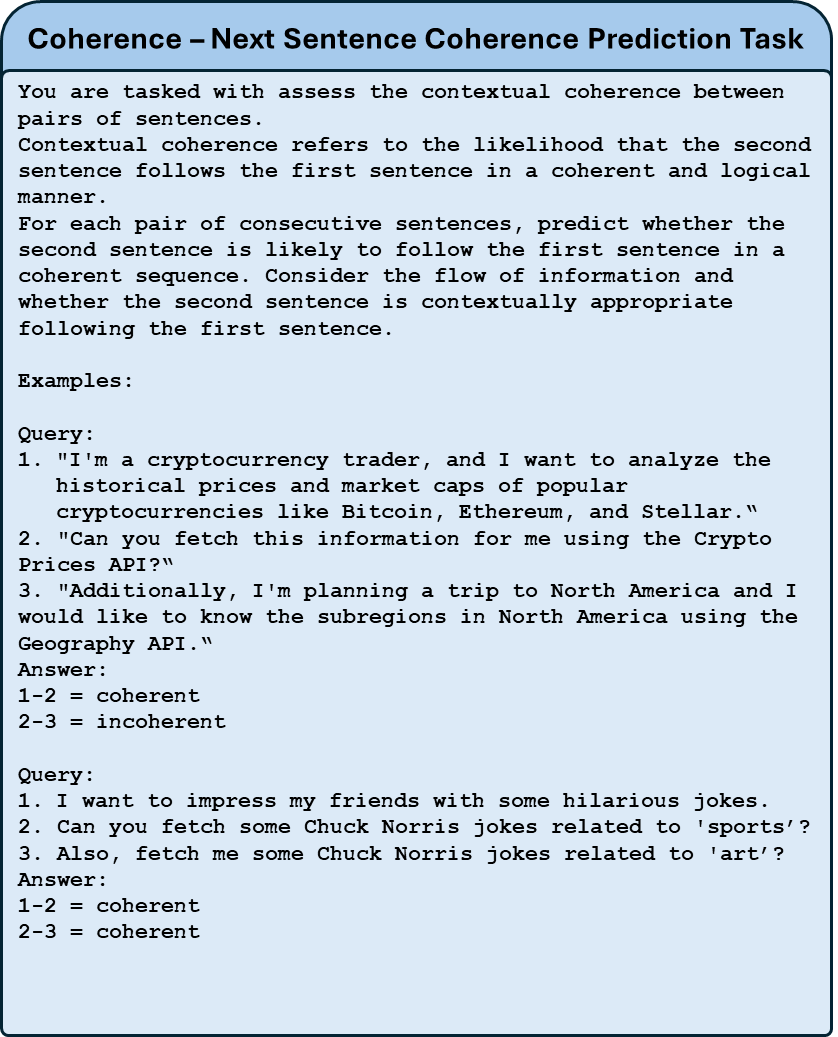}
  \caption{Prompt for Coherence - Next Sentence Coherence Prediction Task. 
  }
  \label{fig:prompt_coherence_task}
\end{figure}

\subsubsection{Solvable}
% \texttt{
% You will be given a user query, and a list of API functions that can return external information.
% Each API function is shown with its domain, name, description, parameters and output fields.
% Determine whether any subset of the API functions could provide all the information required to answer the query.
% No need for one API to answer all the requests in the query, multiple APIs can be used to answer different requests in the query.
% It is alright if a parameter value is not explicitly provided in the query.
% Use the information provided in Domain, Name, Description, and parameters.
% Answer with 'Yes' or 'No' and provide an explanation for your answer.
% Example 1:
% Query: "I'm traveling with my family. Can you tell us what's the weather like in Lisbon for tomorrow? Also, prepare for us an itinerary"
% API Function 1 - Domain: Weather. Name: get\_weather. Description: get weather by city and date. Parameters: city, date. Output: weather\_description.
% API Function 2 - Domain: Traveling. Name: prepare\_itinerary. Description: prepare\_itinerary. Parameters: city, duration. Output: places\_list.
% Explanation: The get\_weather function provides the weather given a city and date. We do not know the date of tomorrow, but we allow non-explicit parameter values. The prepare\_itinerary can handle the second request. Duration is not mentioned, but we allow non-specfic parameters.
% Answer: Yes
% Example 2:
% Query: "Create a video from fashion images"
% API Function 1 - Domain: Content. Name: get\_random\_image. Description: get list of images from the internet. Parameters: query. Output: image.
% API Function 2 - Domain: Content. Name: get\_random\_video. Description: get random video from the internet. Parameters: None. Output: video.
% Explanation: While the first API can get images of fashion, by using free speech query, there is no API function that can create a video from given images.
% Answer: No
% Example 3:
% Query: "Fetch me latest news about NBA"
% API Function 1 - Domain: Sport. Name: get\_statistics. Description: get statistisc of a team. Parameters: team. Output: str.
% API Function 2 - Domain: NBA. Name: get\_news. Description: get latest news. Parameters: None. Output: str.
% Explanation: Looking at API Function 2 Domain 'NBA' we can infer it returns news about the NBA.
% Answer: Yes
% Queries: 
% }
\begin{figure}[h]
  \centering
  \includegraphics[width=\linewidth]{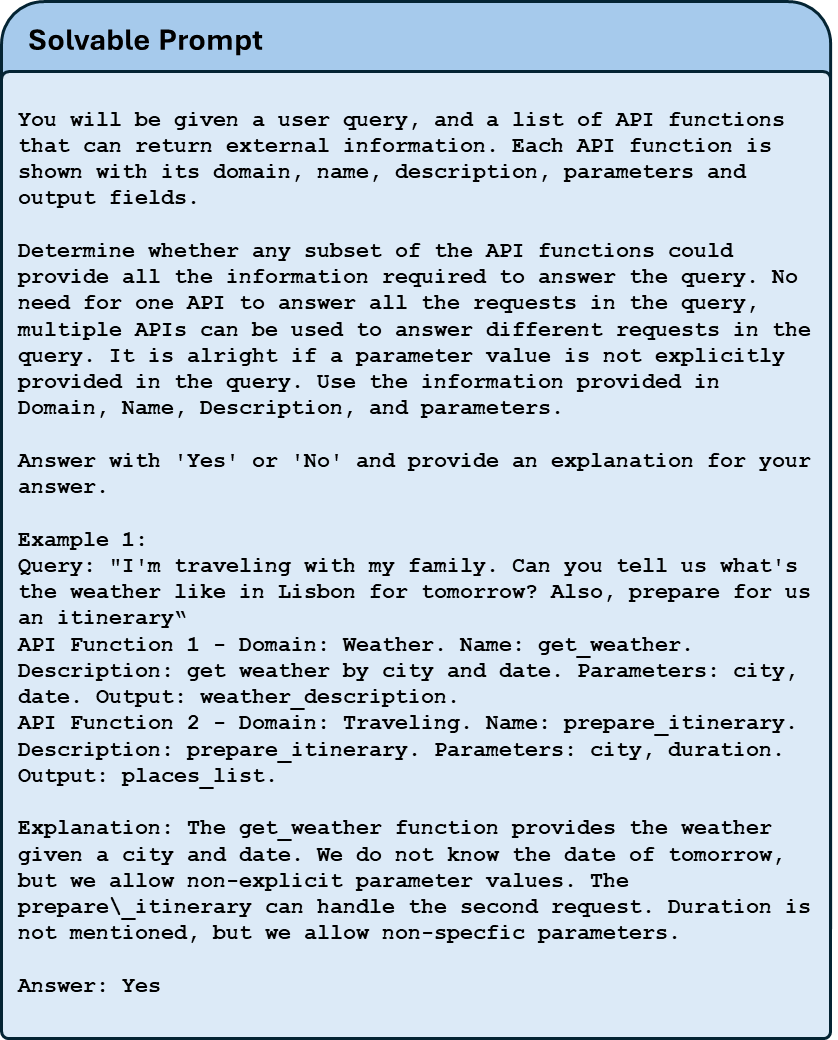}
  \caption{Prompt for Solvable - Direct Questioning. % COMMENT \shadi{What do you think of this?}
  }
  \label{fig:prompt_solvable_direct}
\end{figure}

\subsubsection{Parameters Alignment  - Direct}
% \texttt{
% We need your help in data quality assessment. The data is generated for the goal of training an AI assistant to use API tools.
% You will be given an instruction and API call with parameters. Your task to assess the match quality of called parameters in the provided API calls compared to the specific variables mentioned in the queries, considering the possibility that the api call has added (hallucinated) parameters or the api call has missing called parameters. 
% Rate parameter matching as follows:
% - 3 (High): If the API call parameters fully align with the specific needs mentioned in the query.
% - 2 (Medium): If there is a moderate alignment, low error of added or missing parameters.
% - 1 (Low): If the API call parameters have a low or minimal alignment with the specific needs mentioned in the query, few added parameters not mentioned in the query, or missing parameters mentioned in the query.
% Example:
% Query: "Can you fetch the flight data for the company AZU on June 15th, 2022?"
% API Call: Get\_airline\_data(company = 'AZU', date = '15-6-2022').
% Explanation: company and date parameter values in the API call match the variables mentioned in the query.
% Score: 3 (High).
% Query: "Can you fetch the flight data for the company AZU on June 15th, 2022?"
% API Call: Get\_airline\_data(company = 'AZU').
% Explanation: API Call did not include the date in the called parameters.
% Score: 1 (Low).
% }
\begin{figure}[h]
  \centering
  \includegraphics[width=\linewidth]{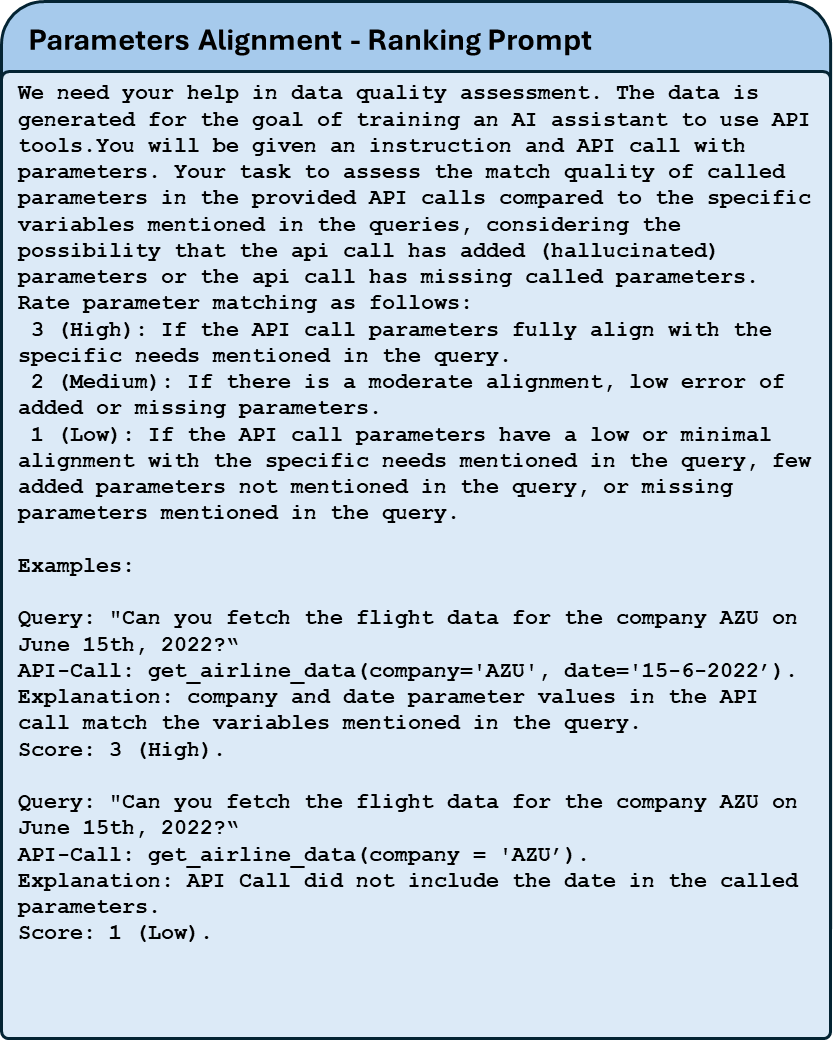}
  \caption{Prompt for Parameters Alignment - Direct Questioning. 
  }
  \label{fig:prompt_param_direct}
\end{figure}


\subsubsection{Parameters Matching - Extraction Task}
% \texttt{
% You will be given a user query, and a list of API functions that are suggested to address the user requests, only a subset of them is relevant to answer the query.
% Each API function is shown with its domain, name, description, parameters and output fields.
% Determine whether the parameter values in the API call sequences are explicitly mentioned in the query.
% In query\_extracted: you have to extract or infer the parameter values from the Query. If a parameter {param1} value is not mentioned in the query write (no\_param1).
% Example 1:
% Query: "I'm traveling with my family. Can you tell us what's the weather like in Lisbon for tomorrow? Also, prepare for us an itinerary"
% Parameters for extraction: [city, date, duration]
% query\_extracted = [city='Lisbon', date='tomorrow', duration='no\_duration']
% Example 2:
% Query: "Create a video from random fashion images"
% Parameters for extraction: [query, date]
% query\_extracted = [query='fashion', date='no\_date']
% Queries: 
% ...
% You will receive sets of parameter names and their corresponding values extracted from queries. Additionally, you will be provided with a sequence of API calls (api\_extracted) along with parameter names and values.
% Your task is to determine whether the parameter values extracted from the queries align with the parameters in the api\_extracted.
% Example 1: 
% query\_extracted = [city='Lisbon', date='17 March', duration='no\_duration'] 
% api\_extracted: [city='Lisbon', date='17-3']
% Explanation: duration value  duration='no\_duration' means it is missing in query\_extracted. It is also missing in api\_extracted. 'Lisbon' in both. Date 17-3 value match but different foramt, which is acceptable.
% answer: Yes
% Example 2:
% query\_extracted = [name='name'] 
% api\_extracted: [name='Suzan']
% Explanation: 'name' and 'Suzan' are different in query\_extracted and api\_extracted. Therefore, not matching.
% answer: No
% Example 3:
% query\_extracted = [] (No parameters to extract)
% api\_extracted: [id='123']
% Explanation: id value is missing in the query\_extracted but not missing in the api call.
% answer: No
% Example 4:
% query\_extracted = [userid='specific userid'] (No parameters to extract)
% api\_extracted: [userid='user123']
% Explanation: 'specific userid' is different than 'user123'. Therefore, not matching
% answer: No
% Follow these giudlines:
% If query\_extracted has no parameters to extract and api\_extracted has no parameters provided, answer with Yes.
% If query\_extracted has (no parameter\_name) and in api\_extracted its provided with a variable parameter\_name=(word), answer with No.
% If query\_extracted has parameter\_name='no\_parameter\_name' and in api\_extracted its provided with a variable parameter\_name='word', answer with No.
% Queries Extraction:
% ...
% }

% \begin{figure}[h]
%   \centering
%   \includegraphics[width=\linewidth]{figures/prompt_param_extract1.png}
%   \caption{Prompt for Parameters Alignment - NLP tasking. Step 1: Extraction Task. 
%   }
%   \label{fig:prompt_param_extract1}
% \end{figure}
% \begin{figure}[h]
%   \centering
%   \includegraphics[width=\linewidth]{figures/prompt_param_compare2.png}
%   \caption{Prompt for Parameters Alignment - NLP tasking. Step 2: Comparison. 
%   }
%   \label{fig:prompt_param_compare2}
% \end{figure}

\begin{figure}[h]
  \centering
  \begin{subfigure}{\linewidth}
    \centering
    \includegraphics[width=0.8\linewidth]{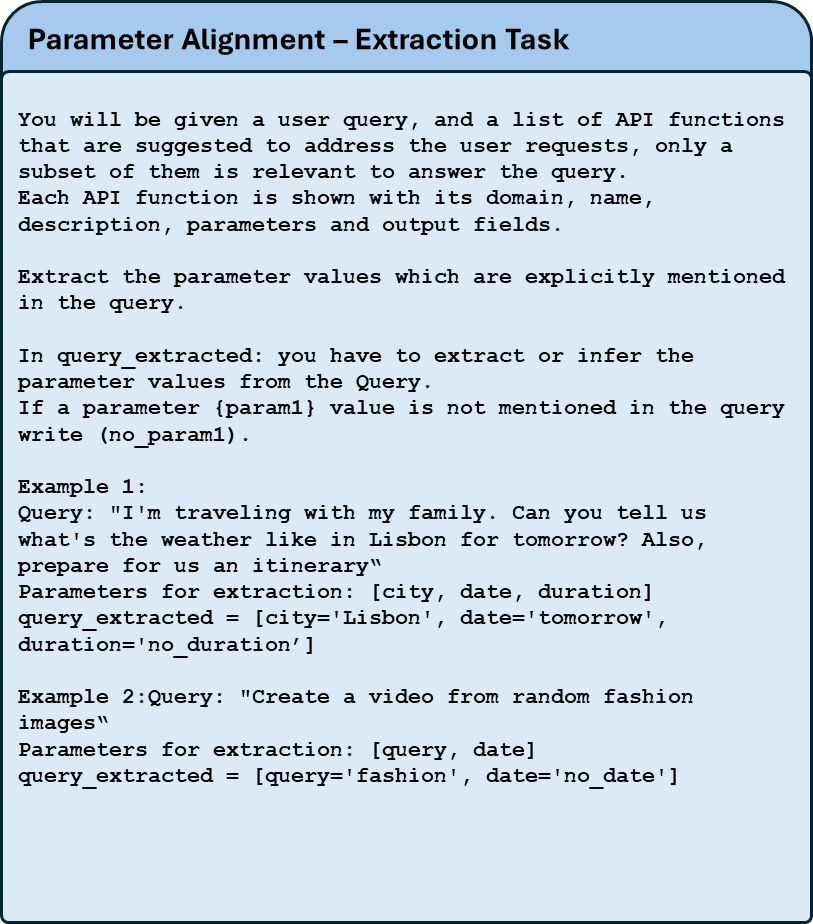}
    \caption{Step 1: Extraction Task.}
    \label{fig:prompt_param_extract1}
  \end{subfigure}
  
  \begin{subfigure}{\linewidth}
    \centering
    \includegraphics[width=0.8\linewidth]{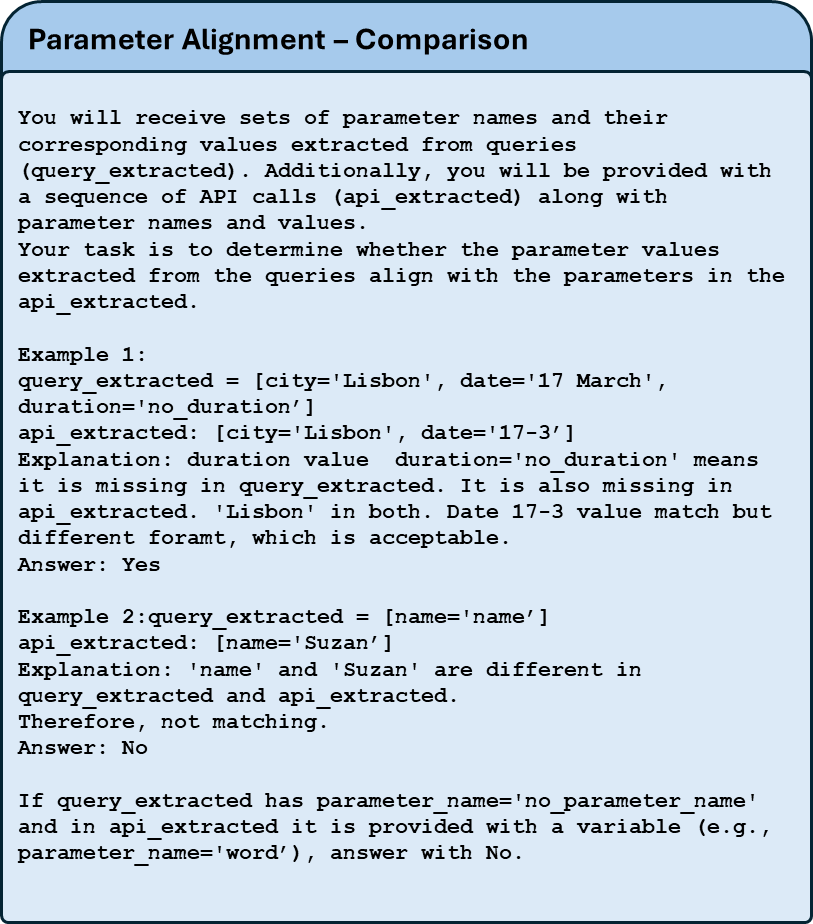}
    \caption{Step 2: Comparison.}
    \label{fig:prompt_param_compare2}
  \end{subfigure}
  
  \caption{Prompt for Parameters Alignment - NLP tasking.}
  \label{fig:prompt_param_task}
\end{figure}

\subsubsection{Matching API sequence + Minimal API calls}
% \texttt{
% You will be given a user query, and a list of API functions that are suggested to address the user requests, only a subset of them is relevant to answer the query.
% Each API function is shown with its domain, name, description, parameters and output fields.
% Determine whether the API call sequences functionality solves the user query with minimal number of calls or it has redundant calls that are not needed to solve the query . 
% Use the information provided in Domain, Name, Description, and parameters. If Description not provided, consider the API as incorrect.
% Each query has multiple requests. The api call sequence should address all different requests.
% Answer with two steps:
% calls\_solves: {Yes/No} whether the API call sequence would fully solve the user query.
% minimal\_calls: {Yes/No} whether the API call sequence solves the user query with minimal number of calls (Yes) or it has redundant calls that are not needed to solve the query (No). 
% Example 1:
% Query: "Can you fetch random fashion images. Then, create a video from these images"
% API call sequence: [get\_random\_image(query='fashion'), get\_video()]
% All APIs Documentation:
% API Function 1 - Domain: Content. Name: get\_random\_image. Description: get list of images from the internet. Parameters: query. Output: image.
% API Function 2 - Domain: Content. Name: get\_video. Description: get trending videos. Parameters: query. Output: video.
% Done Query
% Explanation: get\_random\_image fetches random images. get\_video does not handle the second request of creating video.
% Query calls\_solves: No
% Query minimal\_calls: No
% Example 2:
% Query: "Fetch me latest news about NBA"
% API call sequence: [get\_news(), fetch\_news()]
% API Function 2 - Domain: NBA. Name: get\_news. Description: get latest news. Parameters: None. Output: text.
% API Function 3 - Domain: Finance. Name: fetch\_news. Description: get latest news of trading. Parameters: None. Output: text.
% Done Query
% Explanation: fetch\_news() is redundant, the query does not ask for finance and trading news.
% Query calls\_solves: Yes
% Query minimal\_calls: No
% Queries: 
% ...
% }

\begin{figure}[h]
  \centering
  \includegraphics[width=\linewidth]{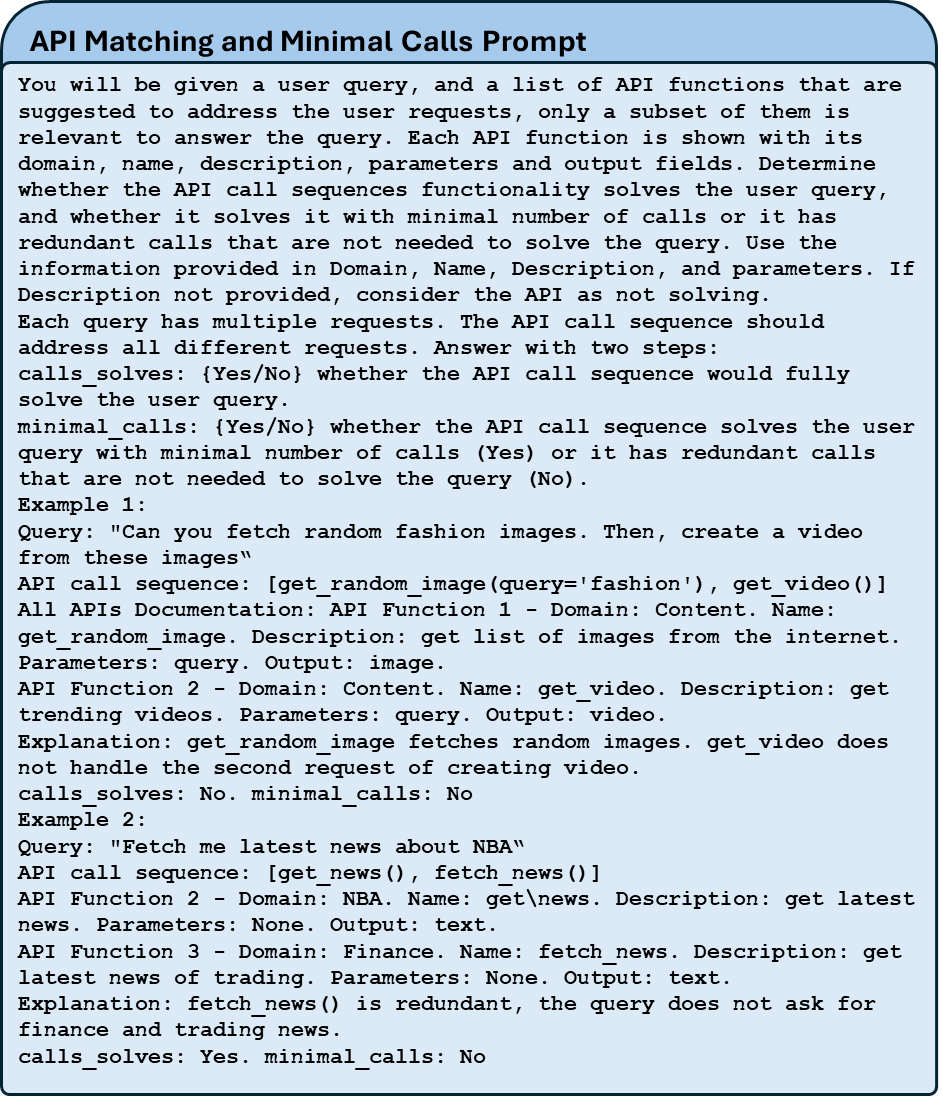}
  \caption{Prompt for API Matching and Minimal Calls. 
  }
  \label{fig:prompt_api}
\end{figure}
